# Supplementary material for: What Can Learned Intrinsic Rewards Capture?
Source: arXiv:1912.05500 source file (2020-08-21)
Supplement: Supplementary file 1 [file supplementary.tex]

%%%%%%%% ICML 2020 EXAMPLE LATEX SUBMISSION FILE %%%%%%%%%%%%%%%%%

\documentclass{article}

% Recommended, but optional, packages for figures and better typesetting:
\usepackage{amssymb}
\usepackage{amsmath}
\usepackage{booktabs} % for professional tables
\usepackage{graphicx}
\usepackage{microtype}
\usepackage{subfig}
\usepackage{pythonhighlight}

% hyperref makes hyperlinks in the resulting PDF.
% If your build breaks (sometimes temporarily if a hyperlink spans a page)
% please comment out the following usepackage line and replace
% \usepackage{icml2020} with \usepackage[nohyperref]{icml2020} above.
\usepackage{hyperref}

% Attempt to make hyperref and algorithmic work together better:

% Optional math commands from https://github.com/goodfeli/dlbook_notation.
\input{math_commands.tex}

% Condensing tricks.

% \newcommand{\revised}[1]{#1}

% Use the following line for the initial blind version submitted for review:
\usepackage[accepted]{icml2020}

% If accepted, instead use the following line for the camera-ready submission:
%\usepackage[accepted]{icml2020}

% The \icmltitle you define below is probably too long as a header.
% Therefore, a short form for the running title is supplied here:
\icmltitlerunning{What Can Learned Intrinsic Rewards Capture?}

\begin{document}

\onecolumn
\icmltitle{Supplementary Material: What Can Learned Intrinsic Rewards Capture?}

% It is OKAY to include author information, even for blind
% submissions: the style file will automatically remove it for you
% unless you've provided the [accepted] option to the icml2020
% package.

% List of affiliations: The first argument should be a (short)
% identifier you will use later to specify author affiliations
% Academic affiliations should list Department, University, City, Region, Country
% Industry affiliations should list Company, City, Region, Country

% You can specify symbols, otherwise they are numbered in order.
% Ideally, you should not use this facility. Affiliations will be numbered
% in order of appearance and this is the preferred way.
\icmlsetsymbol{equal}{*}
\icmlsetsymbol{dagger}{\textdagger}

\begin{icmlauthorlist}
\icmlauthor{Zeyu Zheng}{equal,dagger,michigan}
\icmlauthor{Junhyuk Oh}{equal,dm}
\icmlauthor{Matteo Hessel}{dm}
\icmlauthor{Zhongwen Xu}{dm}
\icmlauthor{Manuel Kroiss}{dm}
\icmlauthor{Hado van Hasselt}{dm}
\icmlauthor{David Silver}{dm}
\icmlauthor{Satinder Singh}{dm}
\end{icmlauthorlist}

\icmlaffiliation{michigan}{University of Michigan}
\icmlaffiliation{dm}{DeepMind}

\icmlcorrespondingauthor{Zeyu Zheng}{zeyu@umich.edu}
\icmlcorrespondingauthor{Junhyuk Oh}{junhyuk@google.com}

% You may provide any keywords that you
% find helpful for describing your paper; these are used to populate
% the "keywords" metadata in the PDF but will not be shown in the document
\icmlkeywords{Machine Learning, ICML}

\printAffiliationsAndNotice{\icmlEqualContribution \textsuperscript{\textdagger}Work done during an internship at DeepMind.} % otherwise use the standard text.

\input{appendix.tex}
%%%%%%%%%%%%%%%%%%%%%%%%%%%%%%%%%%%%%%%%%%%%%%%%%%%%%%%%%%%%%%%%%%%%%%%%%%%%%%%
%%%%%%%%%%%%%%%%%%%%%%%%%%%%%%%%%%%%%%%%%%%%%%%%%%%%%%%%%%%%%%%%%%%%%%%%%%%%%%%

\bibliography{references}
\bibliographystyle{icml2020}

\end{document}
